# Supplementary material for: CYBORGS: Contrastively Bootstrapping Object Representations by Grounding in Segmentation
Source: arXiv:2203.09343 source file (2022-08-16)
Supplement: Supplementary file 1 [file appendix.tex]

\clearpage

% reset Figure number: e.g., Figure B.1.

\setcounter{figure}{0} 
\setcounter{table}{0}

\appendix

\section{Further Method Details and Overview}

Recall in \cref{sec:mask_obj}, to leverage information across a semantic spectrum, we extract features from throughout ResNet-50, instead of using only features from the final convolutional map as in \cite{henaff2021efficient}. Following the notation in \cref{sec:overall} and \cref{sec:mask_obj}, we provide a formal description of this procedure here.

Concretely, given a layer $l$, we define $\vect{y}^{[l]} = f^{[l]}(\vect{v}) \in \mathbb{R}^{D_F \times H_F \times W_F}$ as the feature map of height $H_F$, width $W_F$ and feature resolution $D_F$ obtained at the $l^{th}$ layer of encoding via $f$. Then given a predefined set of layers $\mathcal{L}$, we obtain a final feature map $\mat{F} \in \mathbb{R}^{D_F' \times H_F' \times W_F'}$ via simple layer fusion:

\begin{equation}
\label{eqn:ft_sampling}
    \mat{F} = [S_1(f^{[1]}(\vect{v})); S_2(f^{[2]}(\vect{v})); \cdots ; S_l(f^{[l]}(\vect{v}))], \forall l \in \mathcal{L}
\end{equation}

where $S_l$ is a bilinear upsampling or downsampling layer which projects the feature map at layer $l$ to a desired, common spatial dimensionality $H_F' \times W_F'$ for the concatenation operator $[\cdot\,\,;\,\cdot]$. In our work, we let $\mathcal{L} = \{\texttt{res2}, \texttt{res3}, \texttt{res4}\}$.

We also provide pseudo-code to outline our framework. In \cref{alg:bootstrap}, we detail our KMeans bootstrapping process (c.f. \cref{sec:boot}). In \cref{alg:consistency}, we describe the von Mises-Fisher (vMF) clustering consistency loss (c.f. \cref{sec:curriculum}). Finally, in \cref{alg:main}, we show how these two components fit into the larger framework. Input parameters and hyperparameters are described in the corresponding sections of the main text.

\begin{algorithm}[H]
\caption{Bootstrap segmentation masks (for a single batch of images $\{\mat{I}\}$).}
\label{alg:bootstrap}
\begin{algorithmic}
\Function{BootstrapMasks}{$f_\theta, \{\mat{I}\}, \boldsymbol{\ell}, K_{min}, K_{max}$}
\State Extract feature map $\vect y = f_\theta^{[\boldsymbol{\ell}]} (\{\mat{I}\})$
\State Sample $K \sim Unif(K_{min}, K_{max})$ \Comment{Scale-dynamic sampling}
\State KMeans clustering on $\vect{y}$ with $K$ clusters to obtain feature prototypes $\mat{P}$
\State $\{\mat{M}\} \gets$ Label features in $\vect{y}$ via Euclidean-closest prototype in $\mat{P}$
\State Interpolate $\{\mat{M}\}$ to spatial dimensions of $\{\mat{I}\}$
\State \Return Masks $\{\mat{M}\}$
\EndFunction
% \Statex
\end{algorithmic}
\end{algorithm}
\vspace{-25pt}

\begin{algorithm}[H]
\caption{Clustering consistency loss (for a single batch of images $\{\mat{I}\}$).}
\label{alg:consistency}
\begin{algorithmic}
\Function{ClustConsistency}{$f_\theta, f_\xi, \boldsymbol{\ell}, \{\mat{I}\}, K, \lambda_{loss}$}
\State Augmentations $t \sim \mathcal{T}, t' \sim \mathcal{T'}$
\State $\vect v = t(\{\mat{I}\}), \vect v' = t'(\{\mat{I}\})$
\State Extract feature maps $\vect y = f_\theta^{[\boldsymbol{\ell}]} (\vect{v}), \vect y' = f_\xi^{[\boldsymbol{\ell}]} (\vect{v'})$
\State KMeans clustering on $\vect{y}, \vect{y'}$ with $K$ clusters to obtain feature prototypes $\mat{P}, \mat{P'}$
\State $\mathcal{L} = \lambda_{loss}\mathcal{L}_{clus}$ \Comment{\cref{eqn:consistency}}
\State Update $f_\theta$ to minimize $\mathcal{L}$, $f_\xi$ as EMA of $f_\theta$
\EndFunction
% \Statex
\end{algorithmic}
\end{algorithm}
\vspace{-25pt}

\begin{algorithm}[H]
\caption{CYBORGS Training Flow (for a single batch of images $\{\mat{I}\}$).}
\label{alg:main}
\begin{algorithmic}
\For{$i=1:W$}
\State \Call{ClustConsistency}{$f_\theta, f_\xi, \boldsymbol{\ell}, \{\mat{I}\}, K, 1$} \Comment{vMF warmup period}
\EndFor
\Statex

\State Masks $\{\mat{M}\} = \Call{BootstrapMasks}{f_\theta, \{\mat{I}\}, \boldsymbol{\ell}, K_{min}, K_{max}}$ \Comment{\cref{sec:boot}}
\Statex

\For{$t = W + 1, W + 2, \dots, $}:
\If{$t \,\, \% \,\, N == 0$}
\State Masks $\{\mat{M}\} = \Call{BootstrapMasks}{f_\theta, \{\mat{I}\}, \boldsymbol{\ell}, K_{min}, K_{max}}$
\EndIf
\State Augmentations $t \sim \mathcal{T}, t' \sim \mathcal{T'}$
\State $\vect v = t(\{\mat{I}\}), \vect v' = t'(\{\mat{I}\})$

\State Extract object-level representations $\vect{h_m}, \vect{h'_{m'}}$ using $\{\mat{M}\}$
\Comment{\cref{eqn:ft_pooling}}
\State $\mathcal{L} = \mathcal{L}_{mask}$ \Comment{\cref{eqn:contrast}}
\State Update $f_\theta$ to minimize $\mathcal{L}$, $f_\xi$ as EMA of $f_\theta$
\If{$t \,\, \% \,\, M == 0$}
\State \Call{ClustConsistency}{$f_\theta, f_\xi, \boldsymbol{\ell}, \{\mat{I}\}, K, \lambda_{vMF}$}
\EndIf
\EndFor
\end{algorithmic}
\end{algorithm}

% In short, we first apply the vMF clustering consistency loss during a warmup period ($W$ epochs) for the backbone. We then bootstrap the masks. Finally, in the main pretraining phase, we train the backbone using the available segmentation masks, while periodically using either \cref{alg:bootstrap} (every $N$ epochs) to bootstrap masks or \cref{alg:consistency} (every $M$ epochs) alongside the contrastive objective.

\section{Experimental Details}

\paragraph{Linear transfer.}

We perform linear classification on PASCAL VOC07 and semi-supervised linear transfer on ImageNet-1k, akin to \cite{xie2021unsupervised}. For VOC07, we extract a \emph{frozen} feature map from the penultimate layer of our ResNet-50 pretrained backbone, before downsampling to a $2 \times 2$ spatial grid via adaptive average pooling. We flatten and $\ell2$-normalize the features, yielding $\mathbb{R}^{8192}$ feature vectors. We then train per-class SVMs on the trainval split, performing a 3-fold cross validation on costs $C \in \{0.01, 0.1, 1.0, 10.0\}$, before evaluating mAP on the test split.

For ImageNet-1k, we follow settings from \cite{xie2021unsupervised} and finetune our backbone on the 1\% and 10\% training subset splits as released in \cite{beyer2020we}. We report the top-1 and top-5 accuracy on the official val split.

\paragraph{PASCAL VOC object detection.}

For object detection, we initialize a ResNet-50-C4 backbone with pretrained weights from \app, before inserting into a Faster RCNN architecture. We then finetune with the trainval07+12 split from PASCAL VOC, before reporting all metrics on the test2007 split via the Detectron2 API \cite{wu2019detectron2}. We use all default training settings from \cite{selvaraju2021casting} for standardized comparison.

\paragraph{COCO instance segmentation.}

For segmentation, we initialize a ResNet-50-FPN backbone with pretrained weights from \app, before inserting into a Mask RCNN architecture. We then finetune with the train2017 split from COCO, before reporting all metrics on the val2017 split via the Detectron2 API \cite{wu2019detectron2}. Again, we use all default training settings from \cite{selvaraju2021casting} for standardized comparison, except we follow a 1x training schedule with learning rate decay scheduled accordingly.

\section{Further Semantic Segmentation Results}

\paragraph{CityScapes semantic segmentation}
We further evaluate the segmentation prowess of \app{} representations by transferring to out-of-distribution data. We choose the real-world urban driving scenes CityScapes dataset, and follow the finetuning protocol of \cite{wang2021dense}, training a FCN model on the \texttt{train\_fine} split (2975 images) for 40k iterations before testing on the \texttt{val} split. We demonstrate strong results even when compared to state-of-the-art ImageNet-pretrained SSL methods, suggesting that our bootstrapping of segmentation masks can lead to representations which sensibly adapt to similar segmentation tasks under different data distributions. In particular, we outperform (+0.3 mIoU) \kw{DenseCL} \cite{wang2021dense}, which is a contrastive learning method specifically designed for strong downstream performance on dense prediction tasks, including object detection and semantic segmentation.

\begin{table*}[tb]
    \newcolumntype{Y}{>{\raggedright\arraybackslash}X}

    \centering
    \scriptsize
    \setlength\tabcolsep{1pt}

    \begin{tabularx}{0.55\textwidth}{c l c c c c}
    \toprule
    ~
    & \multicolumn{1}{l}{\bf Method}
    & ~~
    & \multicolumn{1}{l}{\bf Pretraining Data}
    & ~~
    & \multicolumn{1}{l}{\bf mIoU}
    \\
    \midrule
    \ttbf{1)} & \kw{Random Init.} &&
            -- &&
            63.5 \\
            
    \ttbf{2)} & \kw{Supervised} &&
            Supervised, ImageNet &&
            73.7 \\
            
     \midrule
     \ttbf{3)} & \kw{SimCLR} \cite{chen2020simple} &&
            ImageNet &&
            73.1 \\
            
    \ttbf{4)} & \kw{BYOL} \cite{grill2020bootstrap} &&
            ImageNet &&
            71.6 \\
            
    \ttbf{5)} & \kw{MoCo-v2} \cite{chen2020improved} &&
            ImageNet &&
            74.5 \\
            
    \ttbf{6)} & \kw{DenseCL} \cite{wang2021dense} &&
            ImageNet &&
            75.7 \\
    
    \ttbf{7)} & \kw{DetCo} \cite{xie2021detco} &&
            ImageNet &&
            \bf 76.5 \\
     
     \midrule
     \ttbf{8)} & \kw{MoCo-v2} \cite{chen2020improved} &&
            COCO &&
            73.8 \\
            
    \ttbf{9)} & \kw{DenseCL} \cite{wang2021dense} &&
            COCO &&
            75.6 \\
    
    \ttbf{10)} & \kw{BYOL} \cite{grill2020bootstrap} &&
        COCO &&
        72.2 \\
        
    \ttbf{11)} & \kw{ORL} \cite{xie2021unsupervised} &&
        COCO &&
        72.7 \\
    
     \ttbf{12)} & \app (ours) &&
            COCO &&
            \bf 75.9 \\
    
    \bottomrule
    \end{tabularx}
    \setlength{\abovecaptionskip}{5pt plus 3pt minus 2pt}
    \caption{\textbf{Transfer Learning on CityScapes, ResNet-50 backbones.}}
    \label{tab:cityscapes}
    % \vspace{-15pt}
\end{table*}

\paragraph{LVIS long-tail instance segmentation.}

An emerging property of self-supervised representations is their ability to generalize to the semantics of unseen, diverse object distributions \cite{ebert2017self, weng2021unsupervised, tian2021divide}. By assessing transfer performance of \app{} on the LVIS long-tail instance segmentation benchmark, with 1203 object categories across $\sim$164k images \cite{gupta2019lvis}, we hope to verify a similar property in our representations.

\begin{table*}[tb]
    \newcommand{\apbbox}[1]{AP$^\text{\tiny bb}_\text{\tiny #1}$}
    \newcommand{\apmask}[1]{AP$^\text{\tiny mk}_\text{\tiny #1}$}
    \newcolumntype{Y}{>{\raggedright\arraybackslash}X}
    \newcolumntype{Z}{>{\centering\arraybackslash}X}

    \centering
    \scriptsize
    \setlength\tabcolsep{1pt}

    \begin{tabularx}{0.75\textwidth}{c l c c c c c c c c c c YYYYYY}
    \toprule
    ~
    & \multicolumn{1}{l}{\bf \multirow[b]{2}{*}{Method}}
    & ~~
    & \multicolumn{1}{l}{\bf \multirow[b]{2}{*}{\makecell{Pretraining\\ Data}}}
    & ~~~
    & \multicolumn{6}{c}{\bf LVIS, 1x schedule} \\
    \cmidrule{6-11}

    ~ & ~ & ~ & ~ & ~ &
        \apbbox{} & \apbbox{50} & \apbbox{75} &
        \apmask{} & \apmask{50} & \apmask{75} \\
    \midrule
    \ttbf{1)} & \kw{Supervised} &&
                -- &&
                20.4 & 32.9 & 21.7 & 19.4 & 30.6 & 20.5 \\

    \ttbf{2)} & \kw{SoCo} \cite{wei2021aligning} &&
                ImageNet &&
                \bf 26.3 & \bf 41.2 & \bf 27.8 & \bf 25.0 & \bf 38.5 & \bf 26.8 \\  % COCO bbox AP (3) and mask AP (3)
    
     \midrule
     \ttbf{3)} & \kw{DenseCL} \cite{wang2021dense} &&
                COCO &&
                20.0 & 32.3 & 20.9 & 19.7 & 31.0 & 20.8 \\  % COCO bbox AP (3) and mask AP (3)
                
    \ttbf{4)} & \kw{BYOL} \cite{grill2020bootstrap} &&
                COCO &&
                19.8 & 32.6 & 20.8 & 19.4 & 30.5 & 20.5 \\  % COCO bbox AP (3) and mask AP (3)
    
    \ttbf{5)} & \kw{ORL} \cite{xie2021unsupervised} &&
                COCO &&
                20.5 & 33.5 & 21.5 & 20.1 & 31.5 & 21.4 \\  % COCO bbox AP (3) and mask AP (3)
    
     \ttbf{6)} & \app (ours) &&
                COCO &&
                \bf 23.9 & \bf 38.3 & \bf 25.2 & \bf 23.4 & \bf 36.2 & \bf 24.7 \\  % COCO bbox AP (3) and mask AP (3)
    
    \bottomrule
    \end{tabularx}
    \setlength{\abovecaptionskip}{5pt plus 3pt minus 2pt}
    \caption{\textbf{Transfer Learning on LVIS, ResNet-50 backbones.}}
    \label{tab:lvis}
    \vspace{-15pt}
\end{table*}

We follow the standard finetuning protocol in \cite{selvaraju2021casting}, adjusting parameters for a 1x schedule. In comparison to other SSL methods pretrained on COCO, we offer a significant improvement of +3.4 $\text{AP}\textsuperscript{bb}$ and +3.3 $\text{AP}\textsuperscript{mk}$.
